# Supplementary material for: Reversible Electron-Beam Patterning of Colloidal Nanoparticles at Fluid Interfaces
Source: arXiv:2409.08192 ancillary file (2024-09-12)
Supplement: Supplementary file 1 [file SI.pdf]

# Supporting Information for:

## Reversible Electron-Beam Patterning of Colloidal Nanoparticles at Fluid Interfaces

Jonathan G. Raybin,[†,‡] Ethan J. Dunsworth,[¶] Veronica Guo,[§,∥] and Naomi S. Ginsberg[*,†,⊥,#,@,△,∇]

†*Department of Chemistry, University of California, Berkeley, CA 94720, United States.*

‡*Present address: National Insitute of Standards and Technology, Gaithersburg, MD, 20899, United States.*

¶*Department of Engineering Science, University of California, Berkeley, CA 94720, United States.*

§*Department of Physics, University of California, Los Angeles, CA 90024, United States.*

∥*Present address: Department of Physics, Stanford, Stanford, CA, 94305*

⊥*Department of Physics, University of California, Berkeley, CA 94720, United States.*

#*Molecular Biophysics and Integrated Bioimaging Division, Lawrence Berkeley National Laboratory, Berkeley, CA 94720, United States.*

@*Materials Sciences & Chemical Sciences Divisions, Lawrence Berkeley National Laboratory, Berkeley, CA 94720, United States*

△*Kavli Energy NanoScience Institute, Berkeley, CA 94720, United States.*

∇*STROBE, NSF Science & Technology Center, Berkeley, California 94720, United States.*

E-mail: nsginsberg@berkeley.edu

# Supporting Figures and Discussion

## Pattern writing

Examples of colloidal pattern writing with various geometries (**Figure S1**) illustrate the capabilities and limitations of our electron-beam assembly procedure. Each point in the writing sequence involves an independent beam exposure. This approach allows for flexible designs, including patterns composed multiple disconnected elements (**Figure S1c-d)**. This contrasts with colloidal writing techniques that rely on the motion of an ion exchange bead, which are constrained to forming continuous patterns.[1] Each of the patterns shown is created by scanning the electron beam (10 kV; 2.0 $e^-/(\mathrm{nm}^2 \cdot \mathrm{s})$) for periods of 1.8 s (6 frames) at each exposure point. The effective beam attraction collects the 500-nm-diameter particles into features with line widths as low as 8 $\mu$m (16 particle diameters).

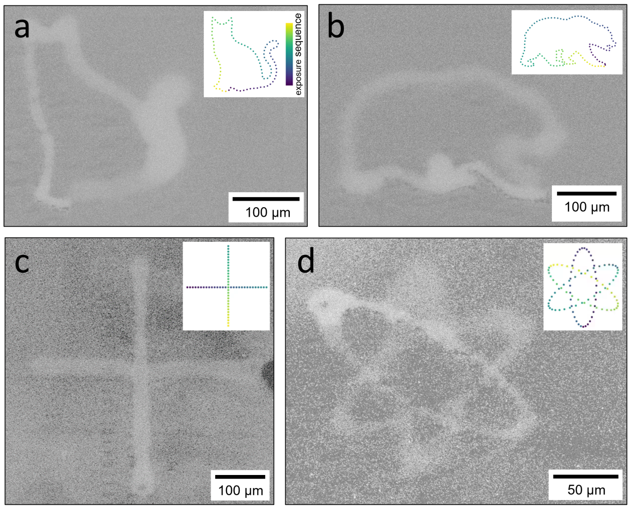


**Figure S1:** Examples of colloidal pattern writing using electron-beam-driven assembly: (a) “cat”, (b) “bear”, (c) “cross”, and (d) “atom” patterns.

In each of these examples, the final pattern is imaged at low magnification, at which individual particles are not resolved, and the electron-scattering contrast arises from variations in colloidal density. At this scale, the low electron flux minimizes disruption to the colloidal organization. Increasing the image magnification for higher resolution imaging induces beam-generated flow, which disrupts the pattern.

Patterning is constrained by the diffusive time scale of the particles. In each of the examples shown, earlier portions of the pattern are significantly broadened by the time that pattern writing is completed. The dissipation time scale is governed by the diffusion of the component particles; for a pattern with $l = 8$ $\mu$m features we estimate a characteristic timescale of $\tau = l^2/D \sim 24.2$ min, consistent with the dissipation rate observed in **Figure 2c** of the main text.

In addition to diffusion, the patterning process itself can lead to distortions if certain effects are not accounted for in pattern design. In general, exposures draw from the same pool of particles, such that increasing the density at one point can reduce the density of the

surrounding area. Each exposure point also induces local solvent currents that can disturb previously patterned areas, especially in feature-dense regions. In our examples, the tightly packed parallel lines in the tail of the "cat" pattern (**Figure S1a**) and the finer details along the outline of the "bear" pattern (**Figure S1b**) both become blurred as a result. In the relatively simple "cross" pattern (**Figure S1c**) the self-intersection is well-defined, but in the more complex "atom" pattern, which has a longer writing time, diffusion causes intersection points to blend together (**Figure S1d**).

Nevertheless, by accounting for these effects during pattern design, we anticipate that blurring and spreading may be minimized. In analogy to error-correction in 3D printing, these factors may corrected either predictively, based on the underlying colloidal physics, or adaptively, through feedback control.[2]

## Péclet number

The Péclet number is a dimensionless transport parameter, defined as the ratio of the advective transport rate to the diffusive transport rate. In terms of Fokker-Planck coefficients, it may be expressed as

$$Pe = \frac{r_{\mathrm{p}}|D_r^{(1)}|}{D_{rr}^{(2)}}, \tag{1}$$

where the particle radius $r_{\mathrm{p}}$ defines the characteristic transport length scale.

In our experiments, the particle response varies across the scan area. Toward the center, particle trajectories are compact and Brownian, and, approaching the edge, they become elongated and are aligned with the radial interaction force (**Figure S2a**). Measurements of $Pe$ show a corresponding crossover from diffusion-dominated transport with $Pe < 1$ to advection-dominated transport with $Pe > 1$ (**Figure S2b**).

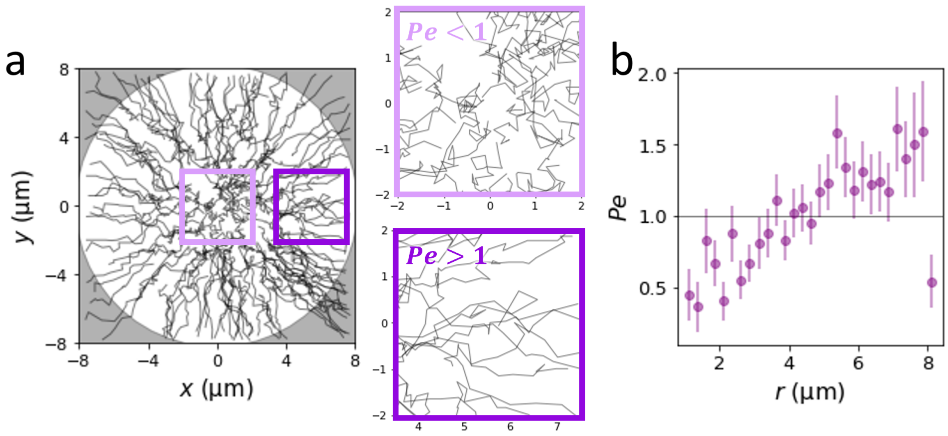


**Figure S2:** Measurement of the Péclet number for particle transport. (a) Particle trajectories transition from diffusion-dominated ($Pe < 1$) at the center of the image (light purple) to advection-dominated ($Pe > 1$) near the edge (dark purple). (b) Variation of $Pe$ within the image area.

# Voltage dependence of colloidal diffusion

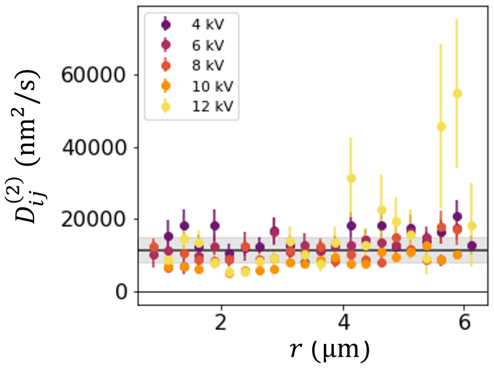


**Figure S3:** Diffusion measurements of 500-nm-diameter particles, corresponding with **Figure 3e** of the main text. Diffusivity is uniform across beam voltages, with $D = 1.1(4) \times 10^{-10}$ cm$^2$/s, consistent with the Stokes-Einstein relation. At 12 kV, measurements near the image edge have high uncertainty due to rapid particle movement toward the center, limiting statistical sampling.

# Glycerol mitigates IL cross-linking

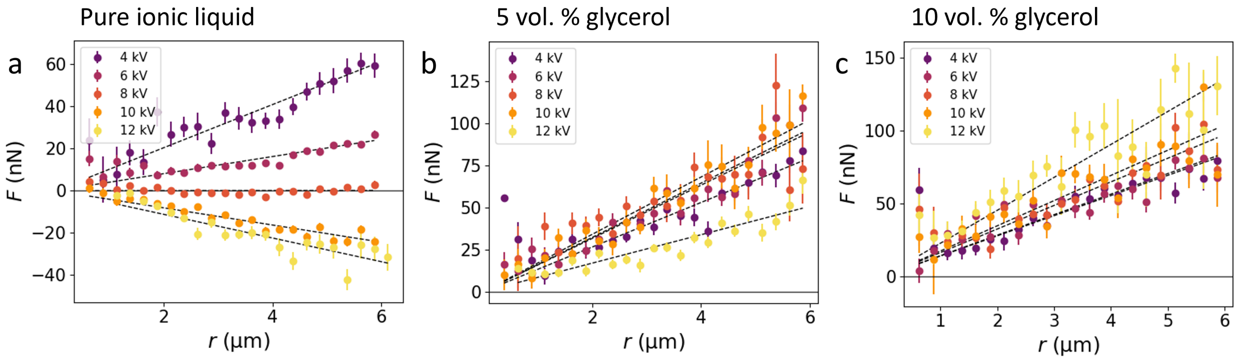


**Figure S4:** Force profile measurements of 300-nm-diameter particles with varying glycerol content in the IL. (a) The beam-particle interaction switches from repulsive to attractive at approximately 8 kV in pure ionic liquid. Consistent repulsion is observed with (b) 5 % and (c) 10 % added glycerol, independent of beam voltage.

## IL flow model

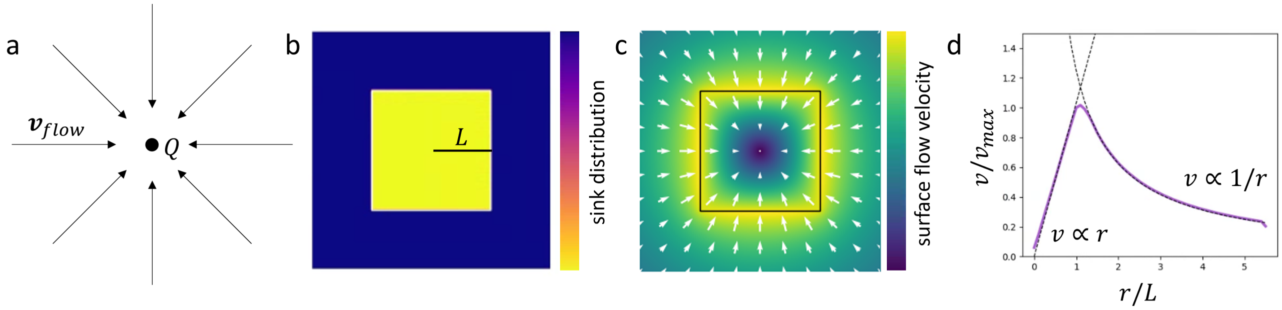


**Figure S5:** Numerical model of the IL flow velocity. (a) Schematic 2D flow converging at a point sink. (b) Electron-beam irradiation is modeled as a uniform sink distribution over the square raster area (side length $2L$), which defines (c) the surface flow velocity field by continuity. (d) Azimuthal averaging shows that the flow velocity scales as $r$ within the image area and $1/r$ outside the image.

In two-dimensional transport, out-of-plane flow is represented by sources or sinks (**Figure S5a**).[3] Flow into a point sink (or from a point source) must satisfy the continuity equation and generates a velocity field:

$$\boldsymbol{v}(x, y) = \pm \frac{Q}{2\pi r} \hat{\boldsymbol{r}}, \tag{2}$$

where $Q$ is the sink (or source) strength, $r = \sqrt{x^2 + y^2}$ is the distance from the point, and $\hat{\boldsymbol{r}}$ is the radial unit vector. More generally, an arbitrary sink distribution $Q(x', y')$ may be represented as a superposition of point sinks and yields a corresponding velocity field:

$$\boldsymbol{v}(x, y) = \iint \frac{Q(x', y')}{2\pi \sqrt{(x - x')^2 + (y - y')^2}} \hat{\boldsymbol{r}} \, dx' \, dy', \tag{3}$$

where $\hat{\boldsymbol{r}}$ is the unit vector in the direction from $(x', y')$ to $(x, y)$, and the integral is taken over the entire distribution.

As a model for the effects of electron-beam irradiation, we assume that the raster pattern yields a square sink distribution (**Figure S5b**) and solve for the flow velocity numerically. The resulting velocity field shows nearly radial symmetry with slight variations near the corners of the box (**Figure S5c**). We note that for radially symmetric (circular) sink distributions, Equation (3) may be solved analytically, and the solutions closely approximate the observed flow pattern. Despite the difference in shape, the modeled velocity field for a square distribution demonstrates similar scaling behavior as a uniform circular distribution, with $v \propto r$ inside the image area and $v \propto 1/r$ outside the exposed region (**Figure S5d**).

# References

(1) Möller, N.; Hecht, L.; Niu, R.; Liebchen, B.; Palberg, T. Writing Into Water. *Small* **2023**, *19*, 2303741.

(2) Brion, D. A. J.; Pattinson, S. W. Generalisable 3D printing error detection and correction via multi-head neural networks. *Nature Communications* **2022**, *13*, 4654.

(3) Faber, T. E. *Fluid Dynamics for Physicists*; Cambridge University Press: Cambridge, 1995.
